# Supplementary material for: DyEdgeGAT: Dynamic Edge via Graph Attention for Early Fault Detection in IIoT Systems
Source: arXiv:2307.03761 source file (2024-01-25)
Supplement: Supplementary file 1 [file 07-appendix.tex]

\appendix
